# Supplementary material for: Systematic study of relativistic and chemical enhancements of $\mathcal{P,T}$-odd effects in polar diatomic radicals
Source: arXiv:1805.05494 ancillary file (2018-06-11)
Supplement: Supplementary file 1 [file suppl.pdf]

# Supplemental Material for "Systematic study of relativistic and chemical enhancements of $\mathcal{P},\mathcal{T}$-odd effects in polar diatomic radicals"

Konstantin Gaul,[1] Sebastian Marquardt,[1] Timur Isaev,[2] and Robert Berger[1]

[1] *Fachbereich Chemie, Philipps-Universität Marburg, Hans-Meerwein-Straße 4, 35032 Marburg, Germany*

[2] *Petersburg Nuclear Physics Institute, Orlova Roscha. 1, 188300 Gatchina, Russia*

(Dated: May 11, 2018)

## I. ALTERNATIVE FORM OF EEDM INTERACTION HAMILTONIAN AND TWO-ELECTRON CONTRIBUTIONS

An alternative expression for the eEDM interaction Hamiltonian, including two-electron interactions implicitly, can be derived:[1, 2]

$$\hat{H}_{\mathrm{d,II}} = \frac{2\imath c d_{\mathrm{e}}}{\hbar e} \sum_{i=1}^{N_{\mathrm{elec}}} \boldsymbol{\gamma}^0 \boldsymbol{\gamma}^5 \hat{\vec{p}}_i^{\,2}. \tag{1}$$

The corresponding ZORA-Hamiltonian is given by[3]:

$$\hat{H}_{\mathrm{d,II}}^{\mathrm{ZORA}} = \imath \hat{\vec{p}}^{\,2} \omega_{\mathrm{d,II}}(\vec{r}) \left( \vec{\boldsymbol{\sigma}} \cdot \hat{\vec{p}} \right) - \imath \left( \vec{\boldsymbol{\sigma}} \cdot \hat{\vec{p}} \right) \omega_{\mathrm{d,II}}(\vec{r}) \hat{\vec{p}}^{\,2}, \tag{2}$$

where the modified ZORA factor is defined as

$$\omega_{\mathrm{d,II}}(\vec{r}) = \frac{2 d_{\mathrm{e}} c^2}{2 e \hbar m_{\mathrm{e}} c^2 - e \hbar \tilde{V}(\vec{r})}. \tag{3}$$

In the following table the deviations of the results of this Hamiltonian from those discussed in our paper are shown for all molecules that are content of our paper. The table shows that two-electron contributions included implicitly in $W_{\mathrm{d,II}}$ are only in super heavy elements noteworthy but always below 10 % and are thus not important for the present discussion.

Table I. Differences between $\mathcal{P},\mathcal{T}$-odd eEDM enhancement in diatomic molecules in a $^2\Sigma_{1/2}$-ground state between two different forms of the interaction operator (Strategem I and II) calculated *ab initio* within a quasi-relativsitc two-component ZORA approach at the cGHF and cGKS/B3LYP level.

| Compound | $Z$ | $W_{\mathrm{d,I}}\,\frac{e\cdot\mathrm{cm}}{10^{24}\cdot h\cdot\mathrm{Hz}}$ cGHF | $W_{\mathrm{d,I}}$ cGKS | $W_{\mathrm{d,II}}\,\frac{e\cdot\mathrm{cm}}{10^{24}\cdot h\cdot\mathrm{Hz}}$ cGHF | $W_{\mathrm{d,II}}$ cGKS | $\Delta_{\mathrm{I/II}}$ cGHF | $\Delta_{\mathrm{I/II}}$ cGKS |
|---|---|---|---|---|---|---|---|
| | | | group 2 fluorides | | | | |
| MgF | 12 | $-4.66\times10^{-2}$ | $-5.22\times10^{-2}$ | $-4.56\times10^{-2}$ | $-5.12\times10^{-2}$ | 2% | 2% |
| CaF | 20 | $-1.47\times10^{-1}$ | $-1.40\times10^{-1}$ | $-1.44\times10^{-1}$ | $-1.38\times10^{-1}$ | 2% | 2% |
| SrF | 38 | $-1.05$ | $-1.01$ | $-1.04$ | $-1.00$ | 1% | 1% |
| BaF | 56 | $-3.32$ | $-2.91$ | $-3.28$ | $-2.87$ | 1% | 1% |
| RaF | 88 | $-2.81\times10^{1}$ | $-2.51\times10^{1}$ | $-2.73\times10^{1}$ | $-2.44\times10^{1}$ | 3% | 3% |
| E120F | 120 | $-3.49\times10^{2}$ | $-3.02\times10^{2}$ | $-3.20\times10^{2}$ | $-2.76\times10^{2}$ | 8% | 8% |
| | | | group 3 oxides | | | | |
| ScO | 21 | $-2.42\times10^{-1}$ | $-1.87\times10^{-1}$ | $-2.38\times10^{-1}$ | $-1.84\times10^{-1}$ | 2% | 2% |
| YO | 39 | $-1.58$ | $-1.32$ | $-1.56$ | $-1.30$ | 1% | 1% |
| LaO | 57 | $-4.82$ | $-3.76$ | $-4.76$ | $-3.71$ | 1% | 1% |
| AcO | 89 | $-4.36\times10^{1}$ | $-3.49\times10^{1}$ | $-4.24\times10^{1}$ | $-3.40\times10^{1}$ | 3% | 3% |
| E121O | 121 | $-6.36\times10^{2}$ | $-4.24\times10^{2}$ | $-5.80\times10^{2}$ | $-3.87\times10^{2}$ | 9% | 9% |
| | | | group 4 nitrides | | | | |
| TiN | 22 | $-4.37\times10^{-1}$ | $-2.06\times10^{-1}$ | $-4.31\times10^{-1}$ | $-2.03\times10^{-1}$ | 1% | 2% |
| ZrN | 40 | $-2.00$ | $-1.36$ | $-1.98$ | $-1.35$ | 1% | 1% |
| HfN | 72 | $-2.93\times10^{1}$ | $-1.59\times10^{1}$ | $-2.88\times10^{1}$ | $-1.56\times10^{1}$ | 2% | 2% |
| RfN | 104 | $3.06\times10^{2}$ | $1.79\times10^{1}$ | $2.91\times10^{2}$ | $1.70\times10^{1}$ | 5% | 5% |
| | | | f-block fluorides | | | | |
| YbF | 70 | $-1.16\times10^{1}$ | $-1.00\times10^{1}$ | $-1.14\times10^{1}$ | $-9.87$ | 2% | 1% |
| NoF | 102 | $-9.69\times10^{1}$ | $-9.77\times10^{1}$ | $-9.26\times10^{1}$ | $-9.34\times10^{1}$ | 4% | 4% |
| | | | f-block oxides | | | | |
| LuO | 71 | $-1.82\times10^{1}$ | $-1.55\times10^{1}$ | $-1.79\times10^{1}$ | $-1.52\times10^{1}$ | 2% | 2% |
| LrO | 103 | $-1.58\times10^{2}$ | $-1.23\times10^{2}$ | $-1.50\times10^{2}$ | $-1.18\times10^{2}$ | 5% | 5% |
| | | | f-block nitrirides | | | | |
| CeN | 58 | $-5.95$ | $-4.34$ | $-5.88$ | $-4.29$ | 1% | 1% |
| ThN | 90 | $-6.16\times10^{1}$ | $-4.65\times10^{1}$ | $-5.98\times10^{1}$ | $-4.51\times10^{1}$ | 3% | 3% |
| | | | group 12 hydrides | | | | |
| ZnH | 30 | $-1.14$ | $-1.10$ | $-1.13$ | $-1.09$ | 1% | 1% |
| CdH | 48 | $-6.36$ | $-5.60$ | $-6.31$ | $-5.55$ | 1% | 1% |
| HgH | 80 | $-8.13\times10^{1}$ | $-5.69\times10^{1}$ | $-7.98\times10^{1}$ | $-5.58\times10^{1}$ | 2% | 2% |
| CnH | 112 | $-1.24\times10^{3}$ | $-6.94\times10^{2}$ | $-1.16\times10^{3}$ | $-6.49\times10^{2}$ | 6% | 6% |
| | | | group 13 oxides | | | | |
| BO | 5 | $9.42\times10^{-3}$ | $1.05\times10^{-2}$ | $9.19\times10^{-3}$ | $1.02\times10^{-2}$ | 2% | 3% |
| AlO | 13 | $-2.13\times10^{-2}$ | $-7.91\times10^{-2}$ | $-2.11\times10^{-2}$ | $-7.77\times10^{-2}$ | 1% | 2% |
| GaO | 31 | $-7.73\times10^{-1}$ | $-1.17$ | $-7.68\times10^{-1}$ | $-1.16$ | 1% | 1% |
| InO | 49 | $-3.76$ | $-4.46$ | $-3.73$ | $-4.42$ | 1% | 1% |
| TlO | 81 | $-5.34\times10^{1}$ | $-3.52\times10^{1}$ | $-5.23\times10^{1}$ | $-3.45\times10^{1}$ | 2% | 2% |

## II. DETERMINATION OF THE COVERAGE REGION IN THE $d_{\mathrm{e}}$,$k_{\mathrm{s}}$-PARAMETER SPACE

In order to disentangle the $\mathcal{P},\mathcal{T}$-odd parameters $k_{\mathrm{s}}$ and $d_{\mathrm{e}}$ at least two experiments with molecules 1 and 2 are needed. The measurement model than is a $2 \times 2$-matrix problem described by the system equations

$$h \begin{pmatrix} \nu_1 \\ \nu_2 \end{pmatrix} = \underbrace{\begin{pmatrix} W_{\mathrm{d},1} & W_{\mathrm{s},1} \\ W_{\mathrm{d},2} & W_{\mathrm{s},2} \end{pmatrix}}_{\mathbf{C}} \begin{pmatrix} d_{\mathrm{e}} \\ k_{\mathrm{s}} \end{pmatrix}, \tag{4}$$

where $\mathbf{C}$ is the matrix of sensitivity coefficients. We follow now Ref. 4 in order to describe the uncertainties and coverage regions determined by two experiments. The covariance matrix $\mathbf{U}_{\mathcal{P},\mathcal{T}}$ of $k_{\mathrm{s}}$ and $d_{\mathrm{e}}$ can be obtained from the covariances of the measured frequencies $\mathbf{U}_\nu$ via the matrix product $\mathbf{C}^{-1}\mathbf{U}_\nu \left(\mathbf{C}^{-1}\right)^T$. Assuming the measurements are uncorrelated $\mathbf{U}_\nu$ is a diagonal matrix with the squared standard uncertainties of the measurements $u^2(\nu_1)$ and $u^2(\nu_2)$ on the diagonal. Thus the covariance matrix $\mathbf{U}_{\mathcal{P},\mathcal{T}}$ has the form

$$\mathbf{U}_{\mathcal{P},\mathcal{T}} = h^2 \begin{pmatrix} \frac{u^2(\nu_1)}{\left(\frac{W_{\mathrm{d},1}}{W_{\mathrm{s},1}} - \frac{W_{\mathrm{d},2}}{W_{\mathrm{s},2}}\right)^2 W_{\mathrm{s},1}^2} + \frac{u^2(\nu_2)}{\left(\frac{W_{\mathrm{d},1}}{W_{\mathrm{s},1}} - \frac{W_{\mathrm{d},2}}{W_{\mathrm{s},2}}\right)^2 W_{\mathrm{s},2}^2} & -\frac{u^2(\nu_1)}{\frac{W_{\mathrm{d},2}}{W_{\mathrm{s},2}}\left(\frac{W_{\mathrm{s},1}}{W_{\mathrm{d},1}} - \frac{W_{\mathrm{s},2}}{W_{\mathrm{d},2}}\right)^2 W_{\mathrm{d},1}^2} - \frac{u^2(\nu_2)}{\frac{W_{\mathrm{d},1}}{W_{\mathrm{s},1}}\left(\frac{W_{\mathrm{s},1}}{W_{\mathrm{d},1}} - \frac{W_{\mathrm{s},2}}{W_{\mathrm{d},2}}\right)^2 W_{\mathrm{d},2}^2} \\ -\frac{u^2(\nu_1)}{\frac{W_{\mathrm{d},2}}{W_{\mathrm{s},2}}\left(\frac{W_{\mathrm{s},1}}{W_{\mathrm{d},1}} - \frac{W_{\mathrm{s},2}}{W_{\mathrm{d},2}}\right)^2 W_{\mathrm{d},1}^2} - \frac{u^2(\nu_2)}{\frac{W_{\mathrm{d},1}}{W_{\mathrm{s},1}}\left(\frac{W_{\mathrm{s},1}}{W_{\mathrm{d},1}} - \frac{W_{\mathrm{s},2}}{W_{\mathrm{d},2}}\right)^2 W_{\mathrm{d},2}^2} & \frac{u^2(\nu_1)}{\left(\frac{W_{\mathrm{s},1}}{W_{\mathrm{d},1}} - \frac{W_{\mathrm{s},2}}{W_{\mathrm{d},2}}\right)^2 W_{\mathrm{d},1}^2} + \frac{u^2(\nu_2)}{\left(\frac{W_{\mathrm{s},1}}{W_{\mathrm{d},1}} - \frac{W_{\mathrm{s},2}}{W_{\mathrm{d},2}}\right)^2 W_{\mathrm{d},2}^2} \end{pmatrix}, \tag{5}$$

where we have expressed the sensitivity factors in terms of the $\mathcal{P},\mathcal{T}$-odd ratios. In order to set tight bounds on both of the $\mathcal{P},\mathcal{T}$-odd parameters the coverage region in the parameter space of $k_{\mathrm{s}}$ and $d_{\mathrm{e}}$ has to become small. We consider now the commonly applied case of an ellipsoidal coverage region. The $\mathcal{P},\mathcal{T}$-odd parameters are characterized by a bivariate Gaussian probability distribution function with $\begin{pmatrix} d_{\mathrm{e}} \\ k_{\mathrm{s}} \end{pmatrix}$ and $\mathbf{U}_{\mathcal{P},\mathcal{T}}$. The ellipse centered at $\begin{pmatrix} d_{\mathrm{e}} \\ k_{\mathrm{s}} \end{pmatrix} = \vec{0}$ is described by

$$\underbrace{\begin{pmatrix} x_{\mathrm{d}} \\ x_{\mathrm{s}} \end{pmatrix}^T \mathbf{U}_{\mathcal{P},\mathcal{T}}^{-1} \begin{pmatrix} x_{\mathrm{d}} \\ x_{\mathrm{s}} \end{pmatrix}}_{f_{\mathrm{e}}(x_{\mathrm{d}},x_{\mathrm{s}})} = k_p^2, \tag{6}$$

where $k_p = 2.45$ for an elliptical region of 95 % probability and $x_{\mathrm{d}}$ and $x_{\mathrm{s}}$ are the coordinates in the parameter space in direction of $d_{\mathrm{e}}$ and $k_{\mathrm{s}}$, respectively. Calculation of the inverse and the products yields an ellipse described by

$$f_{\mathrm{e}}(x_{\mathrm{d}}, x_{\mathrm{s}}) = \left(\frac{W_{\mathrm{d},1}^2}{u^2(\nu_1)} + \frac{W_{\mathrm{d},2}^2}{u^2(\nu_2)}\right) x_{\mathrm{d}}^2 + 2\left(\frac{W_{\mathrm{d},1}^2}{u^2(\nu_1)}\frac{W_{\mathrm{s},1}}{W_{\mathrm{d},1}} + \frac{W_{\mathrm{d},2}^2}{u^2(\nu_2)}\frac{W_{\mathrm{s},2}}{W_{\mathrm{d},2}}\right) x_{\mathrm{d}} x_{\mathrm{s}} + \left(\frac{W_{\mathrm{d},1}^2}{u^2(\nu_1)}\left(\frac{W_{\mathrm{s},1}}{W_{\mathrm{d},1}}\right)^2 + \frac{W_{\mathrm{d},2}^2}{u^2(\nu_2)}\left(\frac{W_{\mathrm{s},2}}{W_{\mathrm{d},2}}\right)^2\right) x_{\mathrm{s}}^2. \tag{7}$$

The area of the ellipse can be readily evaluated via

$$A_{\mathrm{ellipse}} = \frac{2h^2 k_p^2 \pi}{\sqrt{\frac{\partial^2 f_{\mathrm{e}}(x_{\mathrm{d}},x_{\mathrm{s}})}{\partial x_{\mathrm{s}}^2}\frac{\partial^2 f_{\mathrm{e}}(x_{\mathrm{d}},x_{\mathrm{s}})}{\partial x_{\mathrm{d}}^2} - \left(\frac{\partial^2 f_{\mathrm{e}}(x_{\mathrm{d}},x_{\mathrm{s}})}{\partial x_{\mathrm{d}}\partial x_{\mathrm{s}}}\right)^2}} . \tag{8}$$

Thus the ellipse has an area of

$$A_{\mathrm{ellipse}} = \frac{h^2 k_p^2 \pi |u(\nu_1) u(\nu_2)|}{|W_{\mathrm{d},1} W_{\mathrm{d},2}| \left|\frac{W_{\mathrm{s},1}}{W_{\mathrm{d},1}} - \frac{W_{\mathrm{s},2}}{W_{\mathrm{d},2}}\right|} . \tag{9}$$

## III. BASIS SETS

Table II. Basis set parameters for GHF/GKS-ZORA calculations. Even-tempered basis sets of uncontracted Gaussians are given in the form $N_{\mathrm{bas}}\ell$: ($\alpha_{\mathrm{max}}$; $\alpha_{\mathrm{min}}$), where $N_{\mathrm{bas}}$ is the number of Gaussians, $\ell$ is the symbol for the angular momentum quantum numbers and $\alpha_{\mathrm{max}}$ and $\alpha_{\mathrm{min}}$ are the largest and smallest exponent coefficients, respectively, given in units of $a_0^{-2}$ with $a_0$ being the Bohr radius.

| Basis for all 'heavy' centers | | N ANO basis | | |
|---|---|---|---|---|
| | | s | p | d |
| 37s: | (2000000000; 0.0291) | 74761.715 | 126.66657 | 2.7500000 |
| 34p: | (500000000; 0.0582) | 11123.654 | 29.837389 | 0.9625000 |
| 14d: | (13300.758; 0.0521) | 2512.6857 | 9.394038 | 0.3368750 |
| 9f: | (751.8368350; 0.3546) | 703.77729 | 3.405104 | 0.1179060 |
| | | 225.47879 | 1.350000 | |
| | | 79.61581 | 0.5576960 | |
| | | 30.237283 | 0.2324490 | |
| | | 12.263622 | 0.0942640 | |
| | | 5.265086 | 0.0329920 | |
| | | 2.333471 | | |
| | | 0.901856 | | |
| | | 0.358336 | | |
| | | 0.141093 | | |
| | | 0.049383 | | |
| H Dunning basis | | F/O ANO basis | | |
| s | p | s | p | d |
| 82.640 | 2.2920000 | 103109.46 | 245.33029 | 5.000000 |
| 12.410 | 0.8380000 | 15281.007 | 56.919005 | 1.750000 |
| 2.8240 | 0.2920000 | 3441.5392 | 17.604568 | 0.612500 |
| 0.7977 | | 967.09483 | 6.2749950 | 0.214375 |
| 0.2581 | | 314.03534 | 2.4470300 | |
| 0.08989 | | 113.44230 | 0.9950600 | |
| | | 44.644727 | 0.4039730 | |
| | | 18.942874 | 0.1548100 | |
| | | 8.5327430 | 0.0541840 | |
| | | 3.9194010 | | |
| | | 1.5681570 | | |
| | | 0.6232900 | | |
| | | 0.2408610 | | |
| | | 0.0843010 | | |

## IV. SUPPORTING FIGURES

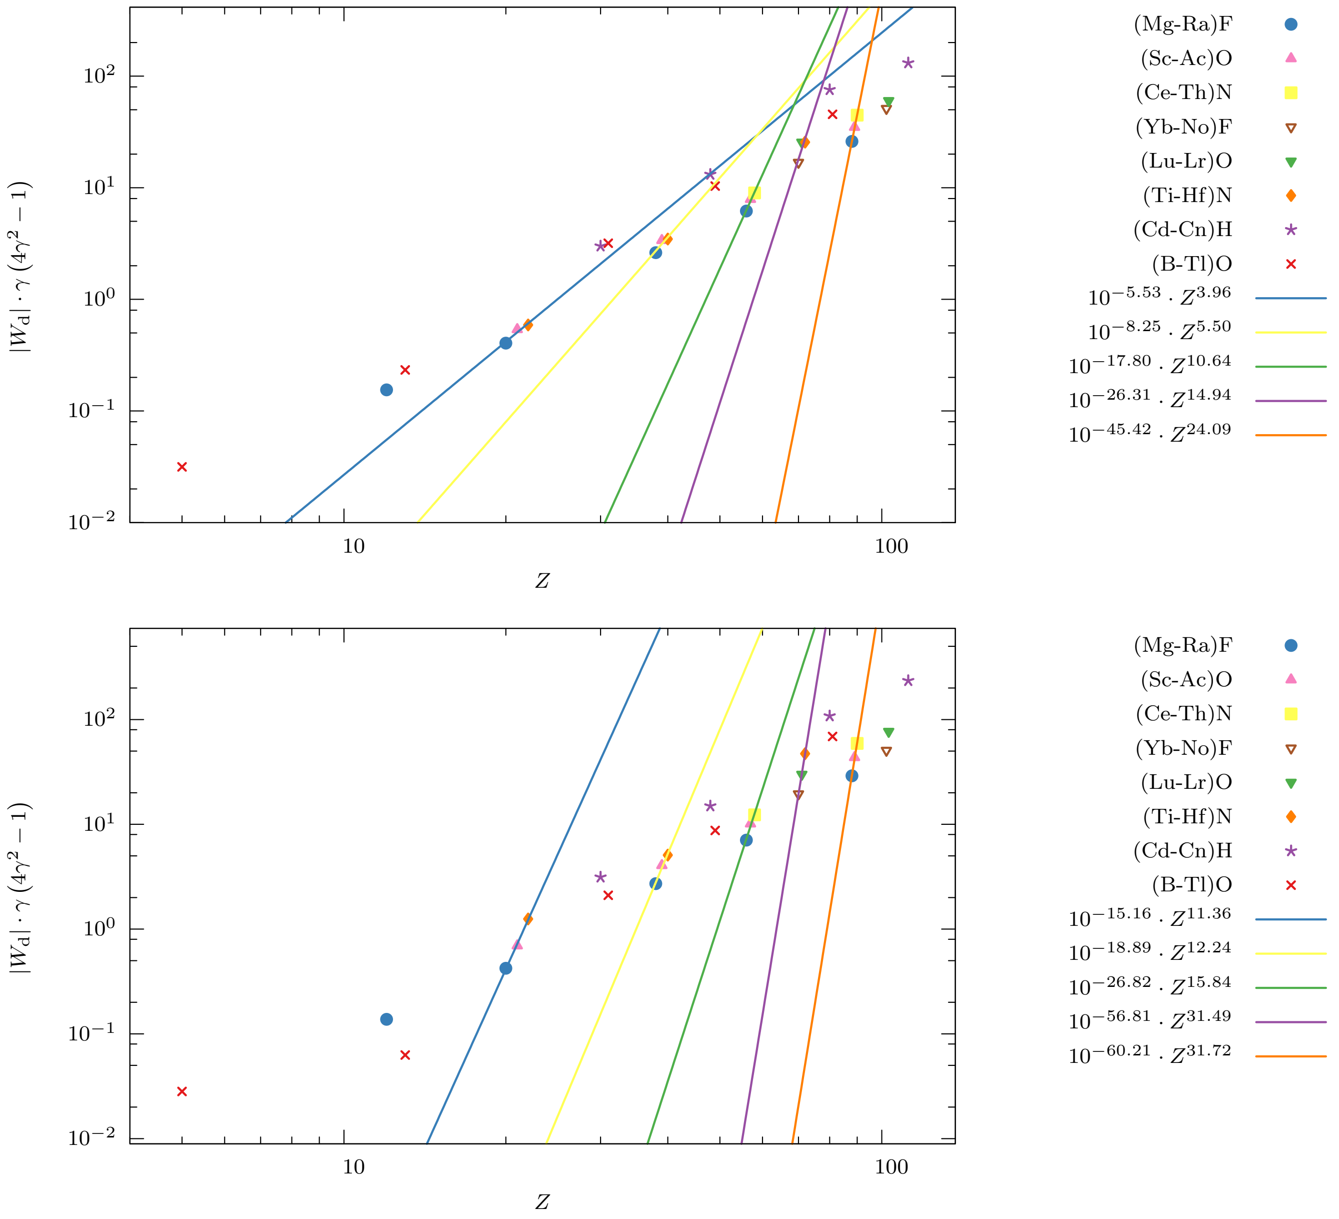


Figure 1. Scaling of $\log_{10}\left\{|W_\mathrm{d}|\gamma\left(4\gamma^2-1\right)\right\}$ with $\log_{10}\{Z\}$ for row 4 (Ca-Ti: blue line), row 5 (Sr-Zr: yellow line), row 6 (Ba-Ce: green line, Yb-Hf: violet line), and row 7 (Ra-Th: organge line) at the level of GKS-ZORA/B3LYP (top) and GHF-ZORA (bottom).

[1] A. Mårtensson-Pendrill and P. Öster, Phys. Scr. **444**, 444 (1987).
[2] E. D. Commins and D. P. DeMille, in *Lept. Dipole Moments*, edited by B. L. Roberts and W. J. Marciano (World Scientific Publishing Company Pte Limited, 2010) p. 519.
[3] K. Gaul and R. Berger, J. Chem. Phys. **147**, 014109 (2017), arXiv:1703.06838 [physics.chem-ph].
[4] JCGM 102:2011, *Evaluation of measurement data  Supplement 2 to the Guide to the expression of uncertainty in measurement  Extension to any number of output quantities* , Standard (Joint Committee for Guides in Metrology, Paris, FR, 2011).
